# Supplementary material for: MemoCRS: Memory-enhanced Sequential Conversational Recommender Systems with Large Language Models
Source: arXiv:2407.04960 source file (2024-07-06)
Supplement: Supplementary file 1 [file appendix.tex]

\appendix
% \footnote{Considering the large API cost of the LLMs, we only conduct experiments on one public dataset.}
\section{Dataset}
Our experiments are conducted on public datasets, MovieLens-1M\footnote{\url{https://grouplens.org/datasets/movielens/1m/}} and Amazon\footnote{\url{https://cseweb.ucsd.edu/~jmcauley/datasets/amazon_v2/}}. \textbf{MovieLens-1M} contains 1 million ratings provided by 6000 users for 4000 movies. Following the data processing similar to DIN~\cite{DIN}, we convert the ratings into binary labels by labeling ratings of 4 and 5 as positive and the rest as negative. The data is split into training and testing sets based on user IDs, with 90\% assigned to the training set and 10\% to the testing set. The dataset contains user features like age, gender, occupation, and item features like item ID and category. The inputs to the models are user features, user behavior history (the sequence of viewed movies with their ID, category, and corresponding ratings), and target item features. \textbf{Amazon-Book}~\cite{ni2019justifying} is the “Books” category of the Amazon Review Dataset. After filtering out the less-interacted users and items, we remain 11, 906 users and 17, 332 items with 1, 406, 582 interactions. The preprocessing is similar to MovieLens-1M, with the difference being the absence of user features. Additionally, ratings of 5 are regarded as positive and the rest as negative.

\section{Backbone Models} Because KAR is a model-agnostic framework, various tasks and models in traditional ID-based recommendation can serve as the backbone model, taking as input the knowledge-augmented vectors generated by KAR. Here, we select two crucial recommendation tasks: \textbf{CTR prediction} and \textbf{reranking}, to validate the effectiveness of KAR across various tasks. CTR prediction aims to anticipate how likely a user is to click on an item, usually used in the ranking stage of recommendation. Reranking is to reorder the items from the previous ranking stage and derive a list that yields more utility and user satisfaction~\cite{liu2022neural}.

We choose 9 representative CTR models as our backbone models, which can be categorized into  user behavior models and feature interaction models. \textbf{User Behavior Models} emphasize modeling sequential dependencies of user behaviors. \textbf{DIN}~\cite{DIN} utilizes attention to model user interests dynamically with respect to a certain item. \textbf{DIEN}~\cite{DIEN} extends DIN by introducing an interest evolving mechanism to capture the dynamic evolution of user interests over time. 

\textbf{Feature Interaction Models} focus on modeling feature interactions between different feature fields. \textbf{DeepFM}~\cite{DeepFM} is a classic CTR model that combines factorization machine (FM) and neural network to capture low-order and high-order feature interactions. \textbf{xDeepFM} \cite{xDeepFM} leverages the power of both deep network and Compressed Interaction Network to generate feature interactions at the vector-wise level. \textbf{DCN}~\cite{DCN} incorporates cross-network architecture and the DNN model to learn the bounded-degree feature interactions. \textbf{DCNv2}~\cite{DCNv2} is an improved framework of DCN which is more practical in large-scale industrial settings. \textbf{FiBiNet}~\cite{FiBiNET} can dynamically learn the feature importance by Squeeze-Excitation network and fine-grained feature interactions by bilinear function. \textbf{FiGNN}~\cite{Fi-GNN} converts feature interactions into modeling node interactions on the graph for modeling feature interactions in an explicit way. \textbf{AutoInt}~\cite{AutoInt} adopts a self-attentive neural network with residual connections to model the feature interactions explicitly.

As fo reranking task, we implement the state-of-the-art models, \eg, \textbf{DLCM}~\cite{ai2018learning}, \textbf{PRM}~\cite{pei2019personalized}, \textbf{SetRank}~\cite{pang2020setrank}, and \textbf{MIR}~\cite{xi2022multi}, as backbone models. \textbf{DLCM} ~\cite{ai2018learning} first applies GRU to encode and rerank the top results. \textbf{PRM}~\cite{pei2019personalized} employs self-attention to model the mutual influence between any pair of items and users' preferences. \textbf{SetRank}~\cite{pang2020setrank} learns permutation-equivariant representations for the inputted items via self-attention. \textbf{MIR} \cite{xi2022multi} models the set-to-list interactions between candidate set and history list with personalized long-short term interests.

\section{PLM-based Baselines}
As for baselines, we compare KAR with methods that leverage pretrained language model to enhance recommendation, such as P5~\cite{p5}, UniSRec~\cite{UniSRec}, VQRec~\cite{VQRec}, TALLRec~\cite{bao2023tallrec}, and LLM2DIN~\cite{harte2023leveraging}. 
\textbf{P5}~\cite{p5} is a text-to-text paradigm that unifies recommendation tasks and learns different tasks with the same language modeling objective during pretraining. \textbf{UniSRec}~\cite{UniSRec} designs a universal sequence representation learning approach for sequential recommenders, which introduces contrastive pretraining tasks to effective transfer across scenarios. 
\textbf{VQ-Rec}~\cite{VQRec} uses Vector-Quantized item representations and a text-to-code-to-representation scheme, achieving effective cross-domain and cross-platform sequential recommendation. \textbf{TALLRec}~\cite{bao2023tallrec} finetunes LLaMa-7B~\cite{llama} with a LoRA architecture on recommendation tasks and enhances the recommendation capabilities of LLMs in few-shot scenarios. In our experiment, we implement TALLRec with LLaMa-2-7B-chat\footnote{https://huggingface.co/meta-llama/Llama-2-7b-chat-hf}, since it has better performance and ability of instruction following. According to~\cite{harte2023leveraging}, we design \textbf{LLM2DIN} which initializes DIN with item
embeddings obtained from chatGLM\cite{du2022glm}. We utilize the publicly available code of these three models and adapt the model to the CTR task with necessary minor modifications. We also align the data and features for all the methods to ensure fair comparisons.

\begin{table}[h]
\centering
% \vspace{-7pt}
\caption{Impact of different knowledge encoders on MoiveLens-1M dataset. 
% LL is short for LogLoss.
% \Jianghao{The best results are given in bold, while the second-best values are underlined.}
}
% \vspace{-5pt}
\scalebox{1.2}{
\setlength{\tabcolsep}{1mm}{
\begin{tabular}{ccc|cc}
\toprule
\multirow{2}{*}{\textbf{Variants}}  & \multicolumn{2}{c|}{\textbf{BERT}} & \multicolumn{2}{c}{\textbf{ChatGLM}} \\
 \cmidrule{2-5}
 & \textbf{AUC} & \textbf{LogLoss} & \textbf{AUC} & \textbf{LogLoss} \\
 \midrule
% base(DIN) & 0.7975 & 0.5387 & 0.7975 & 0.5387  \\
% KAR(LR) & 0.7746 & 0.5699 & 0.7903 & 0.5490  \\
% KAR(MLP) & 0.7882 & 0.5518 & 0.7986 & 0.5399 \\
% KAR-MLP & {\underline{0.8040}} & 0.5345 & 0.8042 & 0.5318  \\
% KAR-MoE & \textbf{0.8046} & \textbf{0.5322} & {\underline{0.8052}} & {\underline{0.5305}}  \\
% KAR & \textbf{0.8046} & {\underline{0.5324}} & \textbf{0.8066} & \textbf{0.5304} \\
base(DIN) & 0.7863 & 0.5486 & 0.7863 & 0.5486 \\
KAR(LR) & 0.7589 & 0.5811 & 0.7720 & 0.5674 \\
KAR(MLP) & 0.7754 & 0.5588 & 0.7816 & 0.5559 \\
KAR-MLP & 0.7934 & 0.5411 & 0.7939 & 0.5401 \\
KAR-MoE & \underline{0.7946} & \textbf{0.5391} & \underline{0.7950} & \underline{0.5394} \\
KAR & \textbf{0.7947} & \underline{0.5402} & \textbf{0.7961} & \textbf{0.5370} \\
\bottomrule
\end{tabular}
}}
% \Jianghao{(1) underline the second best value. (2) significant test is needed}
% \vspace{-5pt}
\label{tab:text_encoder_ml}
\end{table}

\begin{table}[h]
\centering
% \vspace{-7pt}
\caption{Impact of different knowledge encoders on Amazon-Books dataset. 
% LL is short for LogLoss.
% \Jianghao{The best results are given in bold, while the second-best values are underlined.}
}
% \vspace{-5pt}
\scalebox{1.2}{
\setlength{\tabcolsep}{1mm}{
\begin{tabular}{ccc|cc}
\toprule
\multirow{2}{*}{\textbf{Variants}} & \multicolumn{2}{c|}{\textbf{BERT}} & \multicolumn{2}{c}{\textbf{ChatGLM}}  \\
 \cmidrule{2-5}
 & \textbf{AUC} & \textbf{LogLoss} & \textbf{AUC} & \textbf{LogLoss} \\
 \midrule
base(DIN) & 0.8304 & 0.4937 & 0.8304 & 0.4937 \\
KAR(LR)  & 0.7375 & 0.5861 & 0.7560 & 0.5718 \\
KAR(MLP)  & 0.7424 & 0.5834 & 0.7571 & 0.5763 \\
KAR-MLP & 0.8357 & 0.4880 & 0.8370 & 0.4843 \\
KAR-MoE & {\underline{0.8371}} & \textbf{0.4841} & {\underline{0.8388}} & {\underline{0.4823}} \\
KAR & \textbf{0.8374} & {\underline{0.4843}} & \textbf{0.8418} & \textbf{0.4801}\\
\bottomrule
\end{tabular}
}}
% \Jianghao{(1) underline the second best value. (2) significant test is needed}
% \vspace{-5pt}
\label{tab:text_encoder_amz}
\end{table}

\section{Abaltion on Knowledge Encoders and Semantic Transformation}\label{sec:knowledge_encoder}
We employ two different language models, BERT~\cite{bert} and ChatGLM~\cite{du2022glm}, to investigate the impact of different knowledge encoders on model performance. Additionally, we design several variants to demonstrate how the representations generated by knowledge encoders are utilized. \textbf{KAR(LR)} applies average pooling to token representations from the knowledge encoder and directly feeds the result into a linear layer to obtain prediction scores, without utilizing a backbone CTR model. \textbf{KAR(MLP)} replaces the linear layer of KAR(LR) with an MLP. \textbf{KAR-MLP} and \textbf{KAR-MoE} replace the hybrid-expert adaptor with an MLP and a Mixture-of-Experts (MoE), respectively. The original KAR and the two variants, KAR-MLP and KAR-MoE, all adopt DIN as the backbone model. Table~\ref{tab:text_encoder_ml} and~\ref{tab:text_encoder_amz} presents their performance, from which we draw the following conclusions. 

Firstly, we can observe that, overall, variants with ChatGLM as the knowledge encoder outperform those with BERT. The performance of KAR(LR) and KAR(MLP) can be considered as a measure of the quality of the encoded representations, since they directly adopt the representations for prediction. Considering KAR(LR) and KAR(MLP), 
the superior performance of ChatGLM over BERT indicates that ChatGLM performs better in preserving the information within knowledge from LLMs, which may be attributed to the larger size and better text comprehension of ChatGLM (6 billion) compared to BERT (110 million). With ChatGLM on MovieLens-1M, KAR(MLP) is even close to base(DIN), validating the effectiveness of our generated open-world knowledge.
